# Supplementary material for: Water Oxidation Chemistry of Oxynitrides and Oxides: Comparing NaTaO$_3$ and SrTaO$_2$N
Source: arXiv:1806.01252 source file (2018-06-04)
Supplement: Supplementary file 1 [file SupportingInformation.pdf]

**Supporting Information for:**

# Water Oxidation Chemistry of Oxynitrides and Oxides: Comparing $NaTaO_3$ and $SrTaO_2N$

Hassan Ouhbi and Ulrich Aschauer
*Department of Chemistry and Biochemistry, University of Bern, Freiestrasse 3, CH-3012 Bern, Switzerland*
(Dated: May 25, 2018)

## S1. ELECTRONIC AND IONIC STRUCTURE

In Table S1, we show experimental and calculated lattice parameters and band gaps using the PBE functional for $SrTaO_2N$ and for $NaTaO_3$ additionally also with a Hubbard U correction of 2.1 eV applied to the Ta 5$d$ orbitals. We see that both PBE and PBE+U predict lattice parameters that agree with experiment to within 1% and 2% for the oxide and the oxynitride respectively. As expected for a semi-local functional, the band gaps are severely underestimated compared to experiment. Moreover we observe almost no effect of the Hubbard U correction on the band gap.

Table S1. Lattice parameters and band gaps of $SrTaO_2N$ and $NaTaO_3$ calculated with PBE and PBE+U compared to experimental values.

| **Material** | **Method** | **Lattice parameter (Å)** | | | **Band gap (eV)** |
|---|---|---|---|---|---|
| | | **a** | **b** | **c** | |
| $SrTaO_2N$ | PBE | 5.776 | 5.795 | 7.953 | 1.13 |
| | Exp. | 5.694[1] | 5.694[1] | 8.065[1] | 2.1[2] |
| $NaTaO_3$ | PBE | 5.516 | 5.567 | 7.849 | 2.68 |
| | PBE+U | 5.488 | 5.546 | 7.815 | 2.75 |
| | Exp. | 5.476[3] | 5.521[3] | 7.789[3] | 4.1[4] |

In figure S1 we show the projected density of states of the most stable *cis*-a anion order in bulk $SrTaO_2N$ as well as of bulk $NaTaO_3$. While the conduction band is Ta 5$d$ dominated for both materials, the valence band edge of the oxynitride shows mostly N 2$p$ states, whereas the oxide valence band is O 2$p$ dominated.

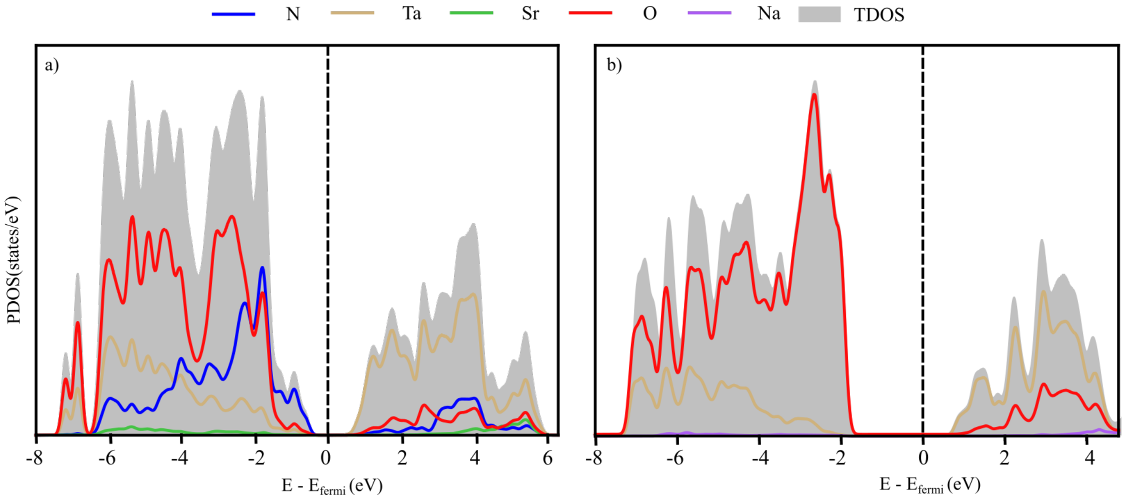


Figure S1. The partial density of states of a) $SrTaO_2N$ *cis*-a and b) $NaTaO_3$ bulk structure

In figure S2 we report the layer-resolved partial density of states of the $NaTaO_3$ (113) surface as well as the two different terminations (SrO and TaON) of the $SrTaO_2N$ (001) surface.

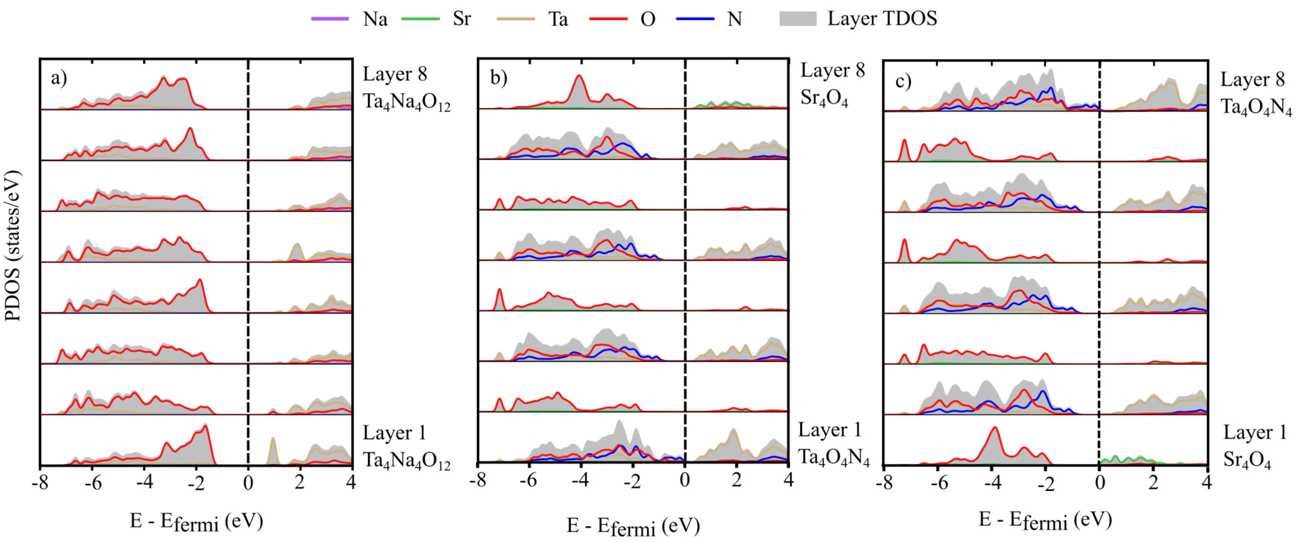


Figure S2. The layer-resolved partial density of states of a) the $NaTaO_3$ (113) $TaNaO_3$ terminated surface as well as the $SrTaO_2N$ (001) surface with b) SrO and c) TaON termination.

## S2. OXYGEN EVOLUTION REACTION

### A. Reaction on single site

The conventional[5] oxygen evolution reaction (OER) mechanism is a succession of four proton-coupled electron transfer reaction steps, where first a water molecule is deprotonated and forms an adsorbed hydroxyl *OH, which is then deprotonated to form an adsorbed oxygen *O. In contact with water a further deprotonation step lead to an adsorbed hydroperoxyl group *OOH, which is released as $O_2$ after a final deprotonation step. This mechanism, which we will refer to as ***mechanism 1***, is detailed in equations 1-4 and can be active on both the A (Na, Sr) and B (Ta) sites.

$$2\,H_2O + * \xrightarrow{A} *OH + H_2O + (H^+ + e^-) \quad (1)$$

$$\xrightarrow{B} *O + H_2O + 2\,(H^+ + e^-) \quad (2)$$

$$\xrightarrow{C} *OOH + 3\,(H^+ + e^-) \quad (3)$$

$$\xrightarrow{D} O_2 + 4\,(H^+ + e^-) \quad (4)$$

In these equations * refers to the active site on the surface (an undercoordinated Ta, Sr or Na), *OH, *O and *OOH are intermediates adsorbed on the active site and A, B, C and D are the labels for water oxidation reaction steps.

The zero-point energy (ZPE) is calculated for each intermediate on the $SrTaO_2N$ (001) surface with TaON termination. The values found in the present work are only slightly different from previously reported ones[6], which means that the magnitude of the ZPE does not vary significantly from one surface to the other. Consequently, we have used the same ZPE for all three surfaces. The entropy of adsorbed molecules was assumed to be zero, while the entropies for gas-phase $H_2O$ and $H_2$ molecules were taken from the JANAF tables at the gas-liquid equilibrium (P=0.035 bar and T=298.15 K)[7].

Table S2. Entropy and zero-point energy of the intermediates species and gas phase molecules.

| Species | TS (eV) | ZPE (eV) |
|---|---|---|
| $H_2O$ | 0.67 | 0.57 |
| $H_2$ | 0.41 | 0.27 |
| *OOH | 0 | 0.45 |
| *OH | 0 | 0.33 |
| *O | 0 | 0.08 |

## B. Reaction on oxygen covered surface

The OER mechanism is found to be different from mechanism 1 (equations 1 to 4) on surfaces covered with *O species as they are predicted under operation conditions by the Pourbaix diagrams shown in the main text. On the *O covered TaON terminated $SrTaO_2N$ (001) surface, the OER occurs via ***mechanism 2*** as detailed in equations 6-9.

$$2\,H_2O + 4\,{*O} \xrightarrow{A} 3\,{*O} + {*HOO} + H_2O + (H^+ + e^-) \quad (5)$$
$$\longrightarrow 4\,{*O} + {*OH} + H_2O + (H^+ + e^-) \quad (6)$$
$$\xrightarrow{B} 4\,{*O} + {*O} + H_2O + 2\,(H^+ + e^-) \quad (7)$$
$$\xrightarrow{C} 4\,{*O} + {*OOH} + 3\,(H^+ + e^-) \quad (8)$$
$$\xrightarrow{D} 4\,{*O} + O_2 + 4\,(H^+ + e^-) \quad (9)$$

In the step A (equation 5) *OOH is unstable, and it is decays into a *O and a *OH as shown by equation 6. On the oxide surface, on which Ta sites are covered by *O, the OER proceeds by ***mechanism 3*** as shown in equations 10-13[8].

$$2\,H_2O + 2\,{*} \xrightarrow{A} {*OH} + H_2O + (H^+ + e^-) \quad (10)$$
$$\xrightarrow{B} 2\,{*OH} + 2\,(H^+ + e^-) \quad (11)$$
$$\xrightarrow{C} {*O} + {*OH} + 3\,(H^+ + e^-) \quad (12)$$
$$\xrightarrow{D} O_2 + 4\,(H^+ + e^-) \quad (13)$$

## C. Reaction free energies

Free energy changes of the various computed OER reaction mechanisms on the three considered surfaces are reported below. Table S3 reports the sum of zero-point energies and entropy contributions for each reaction mechanism. Tables S4 and S5 report the free energy changes of the reaction steps on the oxynitride TaON and SrO termination respectively. Table S6 finally reports the free energy changes for the various reaction steps and different mechanisms on the oxide surface.

Table S3. Sum of zero-point energy ($\Delta$ZPE) and entropy (T$\Delta$S) changes associated with the steps of the different OER mechanisms.

| Step | Mechanism 1 | Mechanism 2 | Mechanism 3 |
|---|---|---|---|
| A | 0.36 | 0.36 | 0.40 |
| B | -0.32 | -0.32 | -0.37 |
| C | 0.40 | 0.40 | 0.39 |
| D | -0.46 | -0.46 | -0.42 |

Table S4. Free energy changes of the various mechanisms on the oxynitride TaON termination. The highlighted cell correspond to the largest free energy change (limiting step) and the value between parentheses is the calculated overpotential for the respective mechanism.

| Step | Mechanism 1 | Mechanism 2 |
|---|---|---|
| A | -0.415 | -0.001 |
| B | 1.360 | 1.179 |
| C | 2.248 (1.018 V) | 2.111 (0.881 V) |
| D | 1.707 | 1.611 |

Table S5. Free energy changes of the various mechanisms on the oxynitride SrO termination. The highlighted cell correspond to the largest free energy change (limiting step) and the value between parentheses is the calculated overpotential for the respective mechanism.

| Step | Mechanism 1 | Mechanism 3 |
|---|---|---|
| A | 0.138 | 0.679 |
| B | 2.370 (1.140 V) | 0.262 |
| C | 1.032 | 0.556 |
| D | 1.361 | 3.403 (2.173) |

Table S6. Free energy changes of the various mechanisms on the oxide surface. The highlighted cell correspond to the largest free energy change (limiting step) and the value between parentheses is the calculated overpotential for the respective mechanism.

| Step | Mechanism 1 | | | Mechanism 1 | Mechanism 3 |
|---|---|---|---|---|---|
| | Na site | Ta site | Na site (Ta *O covered) | Ta site (Ta sites *O covered) | Na sites |
| A | 0.854 | 0.033 | 1.142 | 0.460 | 1.142 |
| B | 2.119 (0.889 V) | 0.827 | 2.220 (0.990 V) | 1.059 | 2.022 (0.792 V) |
| C | 0.704 | 2.530 (1.300 V) | -0.213 | 2.155 (0.925 V) | 0.661 |
| D | 1.223 | 1.510 | 1.750 | 1.225 | 1.074 |

## REFERENCES


[1] B. J. Ennedy, A. K. Prodjosantoso, and C. J. Howard, Journal of Physics: Condensed Matter **11**, 6319 (2006).

[2] T. Takata, C. Pan, and K. Domen, ChemElectroChem **3**, 31 (2016).

[3] S. J. Clarke, K. A. Hardstone, C. W. Michie, and M. J. Rosseinsky, Chemistry of Materials **14**, 2664 (2002).

[4] E. Grabowska, Applied Catalysis B: Environmental **186**, 97 (2016).

[5] J. K. Nørskov, J. Ressmeisl, A. Logadottir, L. Lindqvist, J. R. Kitchin, T. Bligaard, and H. Jonsson, J. Phys. Chem. B **108**, 17886 (2004).

[6] Á. Valdés, Z. W. Qu, G. J. Kroes, J. Rossmeisl, and J. K. Nørskov, Journal of Physical Chemistry C **112**, 9872 (2008).

[7] M. W. Chase, *NIST-JANAF Thermochemical Tables* (American Chemical Society, New York, 1998).

[8] G. Lodi, E. Sivieri, A. De Battisti, and S. Trasatti, Journal of Applied Electrochemistry **8**, 135 (1978).
